# Supplementary material for: Distributed Learning of Neural Lyapunov Functions for Large-Scale Networked Dissipative Systems
Source: arXiv:2207.07731 source file (2022-07-15)
Supplement: Supplementary file 1 [file 07-Appendix.tex]

\appendix
